# Supplementary material for: Enhanced Multi-Resolution Analysis for Multi-Dimensional Data Utilizing Line Filtering Techniques
Source: arXiv:2108.05769 source file (2022-03-10)
Supplement: Supplementary file 3 [file 2D_L-SIAC_Basis_Table.tex]

\begin{landscape}
\begin{table}[h!]
    \centering
    \small
   
    \caption{2D L-SIAC basis functions. For notational convenience suppose $\mathbf{x}$ belongs to element $(i,j)$. }
     \label{tab:2D_LSIAC_basis}
\begin{tabular}{|M{1.5cm}||M{6.5cm}|M{10.5cm}|}\hline
{\bf Region} $S$  & {\bf Basis Function} & {\bf Definition}\\ \hline\hline
  {\bf 1T} &$\chi^{m,r}_{1T,L}(\zeta_x,\zeta_y)$ & $\frac{2-\zeta_y}{2}\int_{-1}^1\phi_{kx}\Big(\zeta_x-\frac{\zeta_y}{2}+\big(1-\frac{\zeta_y}{2}\big)\eta\Big)\phi_{ky}\Big(\big(1-\frac{\zeta_y}{2}\big)\eta+\frac{\zeta_y}{2}\Big)\;d\eta$  \\
   
   &$\chi^{m,r}_{1T,M}(\zeta_x,\zeta_y)$ & $\frac{\zeta_y-\zeta_x}{2}\int_{-1}^1\phi_{kx}\Big(\frac{\zeta_y-\zeta_x}{2}\eta+\frac{\zeta_x-\zeta_y}{2}+1\Big)\phi_{ky}\Big(\frac{\zeta_y-\zeta_x}{2}\eta+\frac{\zeta_y-\zeta_x}{2}-1\Big)\;d\eta$ \\

     &$\chi^{m,r}_{1T,R}(\zeta_x,\zeta_y)$ & $\frac{\zeta_x}{2}\int_{-1}^1\phi_{kx}\Big(\frac{\zeta_x}{2}\eta+\frac{\zeta_x}{2}-1\Big)\phi_{ky}\Big(\frac{\zeta_x}{2}\eta+\zeta_y-1-\frac{\zeta_x}{2}\Big)\;d\eta$ \\ \hline\hline
      
     {\bf 1B} &$\chi^{m,r}_{1B,L}(\zeta_x,\zeta_y)$ & $\frac{2-\zeta_x}{2}\int_{-1}^1\phi_{kx}\Big(\big(1-\frac{\zeta_x}{2}\big)\eta+\frac{\zeta_x}{2}\Big)\phi_{ky}\Big(\zeta_y-\frac{\zeta_x}{2}+\big(1-\frac{\zeta_x}{2}\big)\eta\Big)\;d\eta$  \\
   
     &$\chi^{m,r}_{1B,M}(\zeta_x,\zeta_y)$ & $\frac{\zeta_x-\zeta_y}{2}\int_{-1}^1\phi_{kx}\Big(\frac{\zeta_x-\zeta_y}{2}\eta+\frac{\zeta_x-\zeta_y}{2}-1\Big)\phi_{ky}\Big(\frac{\zeta_x-\zeta_y}{2}\eta+\frac{\zeta_y-\zeta_x}{2}+1\Big)\;d\eta$ \\

       &$\chi^{m,r}_{1B,R}(\zeta_x,\zeta_y)$ & $\frac{\zeta_y}{2}\int_{-1}^1\phi_{kx}\Big(\frac{\zeta_y}{2}\eta+\zeta_x-\frac{\zeta_y}{2}-1\Big)\phi_{ky}\Big(\frac{\zeta_y}{2}\eta-1+\frac{\zeta_y}{2}\Big)\;d\eta$ \\ \hline\hline
      
       {\bf 2T} &$\chi^{m,r}_{2T,L}(\zeta_x,\zeta_y)$ & $-\frac{\zeta_x}{2}\int_{-1}^1\phi_{kx}\Big(-\frac{\zeta_x}{2}\eta+\frac{\zeta_x}{2}+1\Big)\phi_{ky}\Big(-\frac{\zeta_x}{2}\eta+\zeta_y-1-\frac{\zeta_x}{2}\Big)\;d\eta$  \\
   
     &$\chi^{m,r}_{2T,M}(\zeta_x,\zeta_y)$ & $\frac{2+\zeta_x-\zeta_y}{2}\int_{-1}^1\phi_{kx}\Big(\frac{2+\zeta_x-\zeta_y}{2}\eta+\frac{\zeta_x-\zeta_y}{2}\Big)\phi_{ky}\Big(\frac{2+\zeta_x-\zeta_y}{2}\eta+\frac{\zeta_y-\zeta_x}{2}\Big)\;d\eta$ \\

       &$\chi^{m,r}_{2T,R}(\zeta_x,\zeta_y)$ &  $\frac{\zeta_y}{2}\int_{-1}^1\phi_{kx}\Big(\frac{\zeta_y}{2}\eta+\zeta_x-\frac{\zeta_y}{2}+1\Big)\phi_{ky}\Big(\frac{\zeta_y}{2}\eta+\frac{\zeta_y}{2}-1\Big)\;d\eta$ \\ \hline\hline

      {\bf 3T} &$\chi^{m,r}_{3T,L}(\zeta_x,\zeta_y)$ & $-\frac{\zeta_y}{2}\int_{-1}^1\phi_{kx}\Big(-\frac{\zeta_y}{2}\eta-\frac{\zeta_y}{2}+\zeta_x+1\Big)\phi_{ky}\Big(-\frac{\zeta_y}{2}\eta+1+\frac{\zeta_y}{2}\Big)\;d\eta$  \\
   
     &$\chi^{m,r}_{3T,M}(\zeta_x,\zeta_y)$ & $\frac{\zeta_y-\zeta_x}{2}\int_{-1}^1\phi_{kx}\Big(\frac{\zeta_y-\zeta_x}{2}\eta+\frac{\zeta_x-\zeta_y}{2}+1\Big)\phi_{ky}\Big(\frac{\zeta_y-\zeta_x}{2}\eta+\frac{\zeta_y-\zeta_x}{2}-1\Big)\;d\eta$ \\

       &$\chi^{m,r}_{3T,R}(\zeta_x,\zeta_y)$ &  $\frac{2+\zeta_x}{2}\int_{-1}^1\phi_{kx}\Big(\big(\frac{2+\zeta_x}{2}\big)\eta+\frac{\zeta_x}{2}\Big)\phi_{ky}\Big(\big(\frac{2+\zeta_x}{2}\big)\eta-\frac{\zeta_x}{2}+\zeta_y\Big)\;d\eta$ \\ \hline\hline

       {\bf 3B} &$\chi^{m,r}_{3B,L}(\zeta_x,\zeta_y)$ & $-\frac{\zeta_x}{2}\int_{-1}^1\phi_{kx}\Big(-\frac{\zeta_x}{2}\eta+\frac{\zeta_x}{2}+1\Big)\phi_{ky}\Big(-\frac{\zeta_x}{2}\eta+1+\zeta_y-\frac{\zeta_x}{2}\Big)\;d\eta$  \\
   
        &$\chi^{m,r}_{3B,M}(\zeta_x,\zeta_y)$ &  $\frac{\zeta_x-\zeta_y}{2}\int_{-1}^1\phi_{kx}\Big(\frac{\zeta_x-\zeta_y}{2}\eta+\frac{\zeta_x-\zeta_y}{2}-1\Big)\phi_{ky}\Big(\frac{\zeta_x-\zeta_y}{2}\eta+\frac{\zeta_y-\zeta_x}{2}+1\Big)\;d\eta$ \\

        &$\chi^{m,r}_{3B,R}(\zeta_x,\zeta_y)$ &  $\frac{2+\zeta_y}{2}\int_{-1}^1\phi_{kx}\Big(\big(\frac{2+\zeta_y}{2}\big)\eta+\zeta_x-\frac{\zeta_y}{2}\Big)\phi_{ky}\Big(\big(\frac{2+\zeta_y}{2}\big)\eta+\frac{\zeta_y}{2}\Big)\;d\eta$ \\ \hline

     {\bf  4B} &$\chi^{m,r}_{4B,L}(\zeta_x,\zeta_y)$ & $-\frac{\zeta_y}{2}\int_{-1}^1\phi_{kx}\Big(-\frac{\zeta_y}{2}\eta-\frac{\zeta_y}{2}+\zeta_x-1\Big)\phi_{ky}\Big(-\frac{\zeta_y}{2}\eta+1+\frac{\zeta_y}{2}\Big)\;d\eta$  \\
   
       &$\chi^{m,r}_{4B,M}(\zeta_x,\zeta_y)$ & $\frac{\zeta_y-\zeta_x+2}{2}\int_{-1}^1\phi_{kx}\Big(\big(1+\frac{\zeta_y-\zeta_x}{2}\big)\eta+\frac{\zeta_x-\zeta_y}{2}\Big)\phi_{ky}\Big(\big(1+\frac{\zeta_y-\zeta_x}{2}\big)\eta+\frac{\zeta_y-\zeta_x}{2}\Big)\;d\eta$ \\

       &$\chi^{m,r}_{4B,R}(\zeta_x,\zeta_y)$ &  $\frac{\zeta_x}{2}\int_{-1}^1\phi_{kx}\Big(\frac{\zeta_x}{2}\eta+\frac{\zeta_x}{2}-1\Big)\phi_{ky}\Big(\frac{\zeta_x}{2}\eta+1+\zeta_y-\frac{\zeta_x}{2}\Big)\;d\eta$ \\ \hline

\end{tabular}

\end{table}
\end{landscape}
