# Supplementary material for: Enhanced Multi-Resolution Analysis for Multi-Dimensional Data Utilizing Line Filtering Techniques
Source: arXiv:2108.05769 source file (2022-03-10)
Supplement: Supplementary file 7 [file 3D_L-SIAC_Classification_Scheme.tex]

\begin{table}[hp!]
\begin{minipage}[b]{.45\textwidth}
  \centering
          \caption{ Regions present by octant}
          \label{tab:3D_Regions_Present} 
      \begin{tabular}{|c|c|} \hline
           \textbf{Octant}&\textbf{Regions Present} \\ \hline
          \textbf{1} & 1A, 1B, 1C, 1D, 1E, 1F\\ \hline
          \textbf{2} & 2E, 2F\\ \hline
          \textbf{3} & 3A, 3B\\ \hline
          \textbf{4} & 4B, 4F\\ \hline
          \textbf{5}& 5C, 5D\\ \hline
          \textbf{6} & 6D, 6E\\ \hline
          \textbf{7} & 7A, 7C\\ \hline
          \textbf{8} & 8A, 8B, 8C, 8D, 8E, 8F\\ \hline
      \end{tabular}

\end{minipage}\qquad
\begin{minipage}[b]{0.45\textwidth}
  \centering
  \caption{Classification of regions.}
  \label{tab:3D_Classification}
      \begin{tabular}{|c|c|} \hline
           \textbf{Class}&\textbf{Filtering Coordinate Inequality} \\ \hline
          \textbf{(A)} & $\zeta_x\leq\zeta_y\leq\zeta_z$\\ \hline
          \textbf{(B)} & $\zeta_x\leq\zeta_z<\zeta_y$\\ \hline
          \textbf{(C)} & $\zeta_y<\zeta_x\leq\zeta_z$\\ \hline
          \textbf{(D)} & $\zeta_y\leq\zeta_z<\zeta_x$\\ \hline
          \textbf{(E)} & $\zeta_z<\zeta_y\leq\zeta_x$\\ \hline
          \textbf{(F)} & $\zeta_z<\zeta_x<\zeta_y$\\ \hline
      \end{tabular}
\end{minipage}
\end{table}
