# Supplementary material for: Enhanced Multi-Resolution Analysis for Multi-Dimensional Data Utilizing Line Filtering Techniques
Source: arXiv:2108.05769 source file (2022-03-10)
Supplement: Supplementary file 8 [file 3D_L-SIAC_coefficients.tex]

\newpage
  
  \begin{landscape}
  \begin{table}[h!]
      \centering

      \caption{Table describing how the shifting arguments ($q_x,q_y,q_z$) of the $a$ coefficients vary by region.}
      \label{tab:3D_LSIAC_coefficient}
   \begin{tabular}{||M{7.5cm}|M{3cm}|M{3cm}|M{3cm}|M{3cm}||}\hline
\textbf{Region} $\mathbf{S}$ $\mathbf{\Big{\backslash}}$ \textbf{Arguments of} $\mathbf{a_{\alpha}(q_x,q_y,q_z)}$ & $ \mathbf{P=L}$&$ \mathbf{P=LM}$&$ \mathbf{P=RM}$& $\mathbf{P=R}$\\ \hline
\textbf{1A}  &$(0,0,0)$   &  $(0,0,1)$&  $(0,1,1)$ &  $(1,1,1)$  \\ \hline
   
\textbf{1B}  &  $(0,0,0)$   &  $(0,1,0)$&  $(0,1,1)$ &  $(1,1,1)$  \\ \hline
    
\textbf{1C}  &  $(0,0,0)$   &  $(0,0,1)$&  $(1,0,1)$ &  $(1,1,1)$  \\ \hline
\textbf{1D}  &  $(0,0,0)$   &  $(1,0,0)$&  $(1,0,1)$ &  $(1,1,1)$  \\ \hline
\textbf{1E}  &  $(0,0,0)$   &  $(1,0,0)$&  $(1,1,0)$ &  $(1,1,1)$  \\ \hline
   
\textbf{1F}  &  $(0,0,0)$   &  $(0,1,0)$&  $(1,1,0)$ &  $(1,1,1)$  \\ \hline

\textbf{2E}  &  $(0,0,-1)$   &  $(0,0,0)$&  $(1,0,0)$ &  $(1,1,0)$  \\ \hline
   
\textbf{2F}  &  $(0,0,-1)$   &  $(0,0,0)$&  $(0,1,0)$ &  $(1,1,0)$  \\ \hline 

\textbf{3A}  &  $(-1,0,0)$   &  $(0,0,0)$&  $(0,0,1)$ &  $(0,1,1)$  \\ \hline
   
\textbf{3B}  &  $(-1,0,0)$   &  $(0,0,0)$&  $(0,1,0)$ &  $(0,1,1)$  \\ \hline 

\textbf{4B}  &  $(-1,0,-1)$   &  $(-1,0,0)$&  $(0,0,0)$ &  $(0,1,0)$  \\ \hline
   
\textbf{4F}  &  $(-1,0,-1)$   &  $(0,0,-1)$&  $(0,0,0)$ &  $(0,1,0)$  \\ \hline 

\textbf{5C}  &  $(0,-1,0)$   &  $(0,0,0)$&  $(0,0,1)$ &  $(1,0,1)$  \\ \hline
   
\textbf{5D}  &  $(0,-1,0)$   &  $(0,0,0)$&  $(1,0,0)$ &  $(1,0,1)$  \\ \hline 

\textbf{6D}  &  $(0,-1,-1)$   &  $(0,-1,0)$&  $(0,0,0)$ &  $(1,0,0)$  \\ \hline
   
\textbf{6E}  &  $(0,-1,-1)$   &  $(0,0,-1)$&  $(0,0,0)$ &  $(1,0,0)$  \\ \hline

\textbf{7A}  &  $(-1,-1,0)$   &  $(-1,0,0)$&  $(0,0,0)$ &  $(0,0,1)$  \\ \hline
   
\textbf{7C}  &  $(-1,-1,0)$   &  $(0,-1,0)$&  $(0,0,0)$ &  $(0,0,1)$  \\ \hline

\textbf{8A}  &  $(-1,-1,-1)$   &  $(-1,-1,0)$&  $(-1,0,0)$ &  $(0,0,0)$  \\ \hline
   
\textbf{8B}  &  $(-1,-1,-1)$   &  $(-1,0,-1)$&  $(-1,0,0)$ &  $(0,0,0)$  \\ \hline
    
\textbf{8C}  &  $(-1,-1,-1)$   &  $(-1,-1,0)$&  $(0,-1,0)$ &  $(0,0,0)$  \\ \hline
\textbf{8D}  &  $(-1,-1,-1)$   &  $(0,-1,-1)$&  $(0,-1,0)$ &  $(0,0,0)$  \\ \hline
\textbf{8E}  & $(-1,-1,-1)$   &  $(0,-1,-1)$&  $(0,0,-1)$ &  $(0,0,0)$  \\ \hline
   
\textbf{8F}  &  $(-1,-1,-1)$   &  $(-1,0,-1)$&  $(0,0,-1)$ &  $(0,0,0)$  \\ \hline

\end{tabular}

  \end{table}

  \end{landscape}
